# Supplementary material for: Toward a universal foundation model for graph-structured data
Source: arXiv:2604.06391 source file (2026-04-07)
Supplement: Supplementary file 1 [file supplementary_document_main.tex]

\section*{Supporting Information}

% --- Supplementary Fig. 1 (page 1): Class Distribution ---
\begin{figure}[pt]
    \centering
    \includegraphics[width=0.8\linewidth, page=1]{figures/Supplementary_Document_v2.pdf}
    \caption{Class Distribution of different datasets of this study.
    \textbf{a}. PP-Pathways (see Table~\ref{supp_tab:pppathways_classes} for class names) \textbf{b}. HuRI (see Table~\ref{supp_tab:huri_classes} for class names) \textbf{c}. Tabula Muris (see Table~\ref{supp_table:tm_class_name} for class names)
    \textbf{b}. Pan Cancer (Please )see Table~\ref{supp_table:pan_class_name} for class names.
    \textbf{c}. Prostate Cancer.}
    \label{supp_fig:class_distribution}
\end{figure}
%-----------------------------------PPathway------------------------------------

% --- Supplementary Fig. 2 (page 2): PPathway confusion matrix ---
\begin{figure}[pt]
    \centering
    \includegraphics[width=\linewidth, page=2]{figures/Supplementary_Document_v2.pdf}
    \caption{PP-Pathways confusion matrix. Confusion matrix of Graph2Image predictions across 54 cell types with counts shown on a logarithmic colour scale. The prominent diagonal and sparse off-diagonal entries indicate high per-class accuracy with limited cross-class confusion. Class indices and names follow Supplementary Table~\ref{supp_table:tm_class_name}.}
    \label{supp_fig:ppathway_confusion}
\end{figure}

\input{files/ppathway_class_names}

% --- Supplementary Fig. 3 (page 3): PPathway SHAP heatmap ---
\begin{figure}[pt]
    \centering
    \includegraphics[width=0.9\linewidth, page=4]{figures/Supplementary_Document_v2.pdf}
    \caption{Clustered SHAP heatmap revealing tissue-level feature importance structure in the PP-Pathways dataset.
    Clustered heatmap showing normalized SHAP values for the top positively and negatively influential tissues across all PP-Pathways classes. Hierarchical clustering on both tissues (rows) and classes (columns) highlights coherent blocks of shared feature-importance structure. Brain-related tissues form several tight subclusters, reflecting shared expression patterns across related neuroanatomical regions, whereas digestive, reproductive, endocrine, and vascular tissues display distinct SHAP signatures. Columns correspond to PP-Pathways classes, and rows correspond to tissues selected by class-specific SHAP ranking. Color intensity indicates the normalized SHAP magnitude, with red denoting strong positive contributions and blue denoting strong negative contributions. The dual dendrogram structure provides an interpretable overview of how different tissues contribute to Graph2Image model predictions and reveals biologically meaningful relationships among tissue-specific expression profiles.}
    \label{supp_fig:ppathway_shap_heatmap}
\end{figure}

% --- Supplementary Fig. 4 (page 4): PPathway gene dendrogram from SHAP ---
\begin{figure}[pt]
    \centering
    \includegraphics[width=0.9\linewidth, page=3]{figures/Supplementary_Document_v2.pdf}
    \caption{Hierarchical clustering of tissue-level SHAP importance profiles in the PP-Pathways dataset.
    Dendrogram showing the hierarchical relationships among tissues based on their normalized SHAP value profiles across all PP-Pathways classes. Each branch represents a tissue whose SHAP contribution reflects its discriminative importance for class-specific Graph2Image patterns. Tissues with similar SHAP signatures cluster together, revealing shared regulatory or expression landscapes, e.g., anatomically related brain regions and gastrointestinal tissues form coherent subtrees. The clustering is computed using average linkage and Euclidean distance on the top SHAP-ranked features per class. This analysis highlights interpretable groupings of functionally related tissues and provides a global view of how distinct anatomical systems contribute to Graph2Image model predictions.}
    \label{supp_fig:ppathway_dendrogram}
\end{figure}

% --- Supplementary Fig. 5 (page 5): PPathway Class Dendogram ---
\begin{figure}[pt]
    \centering
    \includegraphics[width=0.9\linewidth, page=5]{figures/Supplementary_Document_v2.pdf}
    \caption{Hierarchical clustering of PP-Pathways classes based on normalized SHAP importance profiles.
    Dendrogram illustrating the hierarchical relationships among PP-Pathways classes derived from their normalized SHAP feature-importance signatures. Each leaf corresponds to a tissue class, and branch structure reflects similarity in the SHAP contribution patterns that drive Graph2Image predictions. Closely clustered tissues show highly similar SHAP profiles, revealing biologically coherent groupings, e.g., related brain regions cluster tightly, while immune-associated and gastrointestinal tissues form distinct subtrees. Clustering was performed using average linkage and Euclidean distance on SHAP-selected top features. This visualization provides a global view of class-level similarity in model-derived tissue importance patterns.}
    \label{supp_fig:ppathway_class_dendogram}
\end{figure}

% --- Supplementary Fig. 6 (page 6): PPathway ROC and PR ---
\begin{figure}[pt]
    \centering
    \includegraphics[width=0.9\linewidth, page=6]{figures/Supplementary_Document_v2.pdf}
    \caption{Precision–recall and ROC performance of Graph2Image versus GNN baselines on the PP-Pathways dataset.
    a, Macro-averaged precision–recall curves for Graph2Image and graph neural network baselines (GCN, GAT, GIN, and GraphSAGE). Dashed curves denote F1 contours. Graph2Image achieves substantially higher precision across the full recall range, reflecting stronger discrimination between tissue classes in the PP-Pathways dataset.
    b, ROC curves for the same models. Dashed lines indicate AUC contours. Graph2Image approaches near-perfect sensitivity across false-positive rates, outperforming all GNN baselines. Together, these results highlight the superior separability of Graph2Image embeddings for complex multi-tissue expression signatures.}
    \label{supp_fig:ppathway_roc_pr}
\end{figure}

%--------------------------------------------------HuRI-----------------------------------------
% --- Supplementary Fig. 7 (page 7): PPathway confusion matrix ---
\begin{figure}[pt]
    \centering
    \includegraphics[width=\linewidth, page=7]{figures/Supplementary_Document_v2.pdf}
    \caption{Confusion matrix for Graph2Image predictions on the HuRI dataset.
    Confusion matrix showing classification performance across the nine GTEx-derived tissue classes in the HuRI protein–protein interaction dataset. Graph2Image exhibits strong diagonal dominance, indicating highly accurate tissue-of-origin prediction from gene-level embeddings. Off-diagonal values are minimal across all classes, demonstrating that tissues with distinct expression signatures, i.e., Thyroid, Muscle, Testis and Whole Blood are cleanly separated by the model. Color intensity reflects the number of samples assigned to each true–predicted label pair. Class indices and names follow Supplementary Table~\ref{supp_tab:huri_classes}.}
    \label{supp_fig:huri_confusion}
\end{figure}

\input{files/huri_class_names}

% --- Supplementary Fig. 8 (page 8): Huri gene dendrogram from SHAP ---
\begin{figure}[pt]
    \centering
    \includegraphics[width=0.9\linewidth, page=8]{figures/Supplementary_Document_v2.pdf}
    \caption{Hierarchical clustering of tissue-level SHAP feature importance in the HuRI dataset.
    Dendrogram showing the hierarchical relationships among GTEx tissue features based on their normalized SHAP importance profiles for the HuRI Graph2Image classifier. Each leaf corresponds to a tissue whose SHAP values summarize how strongly that feature contributes to distinguishing the nine HuRI tissue classes. Closely related tissues, such as multiple cortical and cerebellar brain regions or adipose and skin tissues, form coherent subclusters, whereas immune, endocrine and gastrointestinal tissues separate into distinct branches. Distances were computed from SHAP-derived importance vectors using Euclidean distance with average-linkage agglomeration. This analysis indicates that the model’s feature attributions recover biologically meaningful similarity structure among tissues in the HuRI dataset.}
    \label{supp_fig:huri_tissue_dendrogram}
\end{figure}

% --- Supplementary Fig. 9 (page 9): HuRI SHAP heatmap ---
\begin{figure}[pt]
    \centering
    \includegraphics[width=0.9\linewidth, page=9]{figures/Supplementary_Document_v2.pdf}
    \caption{SHAP-based interpretation of Graph2Image predictions on the HuRI interactome.
    Hierarchically clustered heatmap showing the normalized SHAP values for the top predictive genes across the nine GTEx tissues represented in the HuRI–GTEx joint dataset. Rows denote genes selected based on the highest absolute class-specific SHAP contributions, and columns correspond to HuRI tissue classes. Positive SHAP values (red) indicate features that strongly drive the model toward a given tissue prediction, whereas negative values (blue) represent features that oppose that prediction. Dendrograms along both axes reveal that Graph2Image uncovers biologically meaningful co-regulation structure, grouping related tissues (e.g., brain tissues and immune-derived cell types) and clustering coherent gene sets associated with tissue-specific expression programs. The scale bar represents normalized SHAP values.}
    \label{supp_fig:huri_shap_heatmap}
\end{figure}

% --- Supplementary Fig. 10 (page 10): Huri Class Dendogram ---
\begin{figure}[pt]
    \centering
    \includegraphics[width=0.9\linewidth, page=5]{figures/Supplementary_Document_v2.pdf}
    \caption{Hierarchical clustering of tissue-specific SHAP profiles in the HuRI interactome.
    Dendrogram showing hierarchical clustering of the nine HuRI tissue classes based on their normalized SHAP importance profiles derived from Graph2Image embeddings. Distances reflect similarity in feature attribution patterns across tissues, revealing biologically meaningful groupings such as the close proximity of brain regions (Cerebellum and Cerebellar Hemisphere), immune-related cell types (EBV-transformed lymphocytes and cultured fibroblasts), and reproductive tissues (Ovary and Testis). Clustering was performed using average linkage and Euclidean distance.}
    \label{supp_fig:huri_class_dendogram}
\end{figure}

% --- Supplementary Fig. 11 (page 11): Huri ROC and PR ---
\begin{figure}[pt]
    \centering
    \includegraphics[width=0.9\linewidth, page=11]{figures/Supplementary_Document_v2.pdf}
    \caption{Performance comparison of Graph2Image and graph neural network baselines on the HuRI interactome.
    a, Micro-averaged precision–recall curves for Graph2Image and baseline GNNs (GCN, GAT, GIN, GraphSAGE) on the nine-class HuRI tissue classification task. Graph2Image achieves consistently higher precision across the full recall range, indicating stronger discriminative ability in this sparse interactome setting.
    b, ROC curves showing that Graph2Image attains markedly higher true-positive rates at low false-positive rates, reflecting improved sensitivity. Dashed lines denote F1 (panel a) and AUROC (panel b) reference contours for visual calibration.}
    \label{supp_fig:huri_roc_pr}
\end{figure}

\input{files/huri_gene_names}

% --- Supplementary Fig. 12 (page 12): TM confusion matrix ---
\begin{figure}[pt]
    \centering
    \includegraphics[width=0.75\linewidth, page=12]{figures/Supplementary_Document_v2.pdf}
    \caption{Tabula Muris confusion matrix. Confusion matrix of Graph2Image predictions across 55 cell types with counts shown on a logarithmic colour scale. The prominent diagonal and sparse off-diagonal entries indicate high per-class accuracy with limited cross-class confusion. Class indices and names follow Supplementary Table~\ref{supp_table:tm_class_name}.}
    \label{supp_fig:tm_confusion}
\end{figure}

% --- Supplementary Fig. 13 (page 13): TM dendrogram from SHAP ---
\begin{figure}[pt]
    \centering
    \includegraphics[width=0.75\linewidth, page=13]{figures/Supplementary_Document_v2.pdf}
    \caption{Tabula Muris dendrogram from SHAP profiles. Hierarchical clustering of the 55 cell types using class-averaged, gene-level SHAP profiles (average-linkage, Euclidean distance). The branching recapitulates expected haematopoietic and epithelial lineages and reveals coherent groupings discussed in the main text.}
    \label{supp_fig:tm_dendrogram}
\end{figure}

% --- Supplementary Fig. 14 (page 14): TM SHAP heatmap ---
\begin{figure}[pt]
    \centering
    \includegraphics[width=0.75\linewidth, page=14]{figures/Supplementary_Document_v2.pdf}
    \caption{Tabula Muris class-averaged SHAP heatmap. Heatmap of class-averaged SHAP values for top marker genes across all 55 cell types. SHAP values are normalised within each class to the maximum absolute value; warm colours denote features increasing class probability and cool colours the converse. Gene names are listed in Supplementary Table~\ref{supp_table:tm_shap_genes_part_1}, \ref{supp_table:tm_shap_genes_part_2}, and \ref{supp_table:tm_shap_genes_part_3}; cell-type labels follow Supplementary Table~\ref{supp_table:tm_class_name}.}
    \label{supp_fig:tm_shap_heatmap}
\end{figure}

\input{files/tm_class_names}
\input{files/tm_gene_dendogram}

% --- Supplementary Fig. 15 (page 15): Pan-cancer confusion matrix ---
\begin{figure}[pt]
    \centering
    \includegraphics[width=0.9\linewidth, page=15]{figures/Supplementary_Document_v2.pdf}
    \caption{Pan-cancer confusion matrix. Confusion matrix of Graph2Image predictions across 32 TCGA cancer types with a logarithmic colour scale. The strong diagonal highlights accurate class assignment, while rare off-diagonal entries capture confusions among related tissues. Cancer-type names and order follow Supplementary Table~\ref{supp_table:pan_class_name}.}
    \label{supp_fig:pan_confusion}
\end{figure}

% --- Supplementary Fig. 16 (page 16): Pan-cancer SHAP heatmap ---
\begin{figure}[pt]
    \centering
    \includegraphics[width=0.8\linewidth, page=16]{figures/Supplementary_Document_v2.pdf}
    \caption{Pan-cancer class-averaged SHAP heatmap. Heatmap of class-averaged SHAP values for mRNA features across 32 cancer types, normalised within class (max $|$SHAP$|=1$). Distinct blocks reflect shared transcriptional programmes and cancer-type-specific signatures described in the main text. Gene names are provided in Supplementary Table~\ref{supp_table:pan_shap_genes_part_1} and \ref{supp_table:pan_shap_genes_part_2}; labels follow Supplementary Table~\ref{supp_table:pan_class_name}.}
    \label{supp_fig:pan_shap_heatmap}
\end{figure}

% --- Supplementary Fig. 17 (page 17): Omics contributions via SHAP ---
\begin{figure}[pt]
    \centering
    \includegraphics[width=0.8\linewidth, page=17]{figures/Supplementary_Document_v2.pdf}
    \caption{Relative contribution of omics modalities. Per-class mean absolute SHAP partitioned by mRNA, copy-number variation (CNV) and DNA methylation for each cancer type. Modality usage mirrors tissue of origin and known driver biology. Cancer-type order matches Supplementary Table~\ref{supp_table:pan_class_name}.}
    \label{supp_fig:pan_modal_contrib}
\end{figure}

% --- Supplementary Fig. 18 (page 18): Pan-cancer dendrogram from SHAP ---
\begin{figure}[pt]
    \centering
    \includegraphics[width=0.8\linewidth, page=18]{figures/Supplementary_Document_v2.pdf}
    \caption{Pan-cancer dendrogram from SHAP profiles. Hierarchical clustering of 32 cancer types using class-level SHAP profiles (average-linkage, Euclidean distance). The arrangement groups tumours with shared molecular programmes and anatomical origin; salient clades are discussed in the main text.}
    \label{supp_fig:pan_dendrogram}
\end{figure}

\input{files/pan_label_abbreviation}
\input{files/pan_labels}
\input{files/pan_gene_list}

% --- Supplementary Fig. 19 (page 19): Prostate butterfly plots ---
\begin{figure}[pt]
    \centering
    \includegraphics[width=0.9\linewidth, page=9]{figures/Supplementary_Document_v2.pdf}
    \caption{‘Butterfly’ plots of gene-level SHAP in prostate cancer. Mirrored kernel-density estimates of SHAP distributions for selected genes in primary versus metastatic tumours highlight features that preferentially drive each state. Genes are ordered by cohort-wide importance.}
    \label{supp_fig:pnet_butterfly}
\end{figure}

% --- Supplementary Fig. 20 (page 20): Prostate gene dendrogram ---
\begin{figure}[pt]
    \centering
    \includegraphics[width=0.85\linewidth, page=20]{figures/Supplementary_Document_v2.pdf}
    \caption{Prostate cancer gene dendrogram from SHAP profiles. Average-linkage clustering (Euclidean distance) of top predictive genes using their SHAP profiles across samples identifies modules associated with primary or metastatic disease states. Gene names are the supplementary Table~\ref{supp_table:pnet_gene_dendrogram_key}.}
    \label{supp_fig:pnet_gene_dendrogram}
\end{figure}

\input{files/pnet_gene_dendogram}

\FloatBarrier
\section{Clustering Metrics}
To assess the quality of the embedding spaces learned by each model, we used a set of standard clustering metrics that compare the learned clusters to the known biological labels. The adjusted Rand index (ARI) measures how often pairs of samples are grouped together or separated in the same way as the ground-truth labels, while correcting for random agreement. Normalized mutual information (NMI) quantifies how much information about the true labels is preserved by the clustering, and is insensitive to the absolute number of clusters.

We further report homogeneity and completeness to characterize the purity of clusters from two complementary perspectives. Homogeneity measures whether each predicted cluster contains samples from only a single true class, whereas completeness measures whether all samples from a given class are assigned to the same cluster. The V-measure is the harmonic mean of homogeneity and completeness, and it summarizes the trade-off between these two properties.

Finally, we compute the silhouette coefficient directly in the embedding space. This metric compares the average distance of each sample to points in the same cluster versus points in the nearest different cluster. High silhouette scores indicate compact, well-separated clusters in the underlying feature space, independent of the label information. Taken together, these metrics allow us to evaluate both label alignment (ARI, NMI, homogeneity, completeness, V-measure) and geometric separation (silhouette) of the learned embeddings.

Let $\mathcal{U} = \{U_1,\dots,U_R\}$ be the ground–truth partition of $N$ samples
and $\mathcal{V} = \{V_1,\dots,V_C\}$ be the clustering obtained from an
embedding (e.g.\ Graph2Image or a GNN).  
Define the contingency table
\[
n_{ij} = |U_i \cap V_j|, \qquad
a_i = \sum_{j} n_{ij}, \qquad
b_j = \sum_{i} n_{ij}, \qquad
N = \sum_{i,j} n_{ij},
\]
and denote the binomial coefficient by
$\binom{n}{2} = \frac{n(n-1)}{2}$.

\subsection*{Adjusted Rand Index (ARI)}

The Rand index measures the agreement between two partitions in terms of
pairwise co–assignment.  The adjusted Rand index corrects this quantity
for chance:
\begin{equation}
\mathrm{ARI}(\mathcal{U},\mathcal{V})
=
\frac{
    \displaystyle
    \sum_{i,j} \binom{n_{ij}}{2}
    -
    \frac{
        \left(\displaystyle\sum_{i} \binom{a_i}{2}\right)
        \left(\displaystyle\sum_{j} \binom{b_j}{2}\right)
    }{\binom{N}{2}}
}{
    \displaystyle
    \tfrac{1}{2}
    \left[
        \sum_{i} \binom{a_i}{2}
        +
        \sum_{j} \binom{b_j}{2}
    \right]
    -
    \frac{
        \left(\displaystyle\sum_{i} \binom{a_i}{2}\right)
        \left(\displaystyle\sum_{j} \binom{b_j}{2}\right)
    }{\binom{N}{2}}
}.
\end{equation}
$\mathrm{ARI}=1$ indicates perfect agreement and $\mathrm{ARI}\approx 0$
corresponds to random labeling (negative values are possible when the
agreement is worse than random).

\subsection*{Normalized Mutual Information (NMI)}

The mutual information between $\mathcal{U}$ and $\mathcal{V}$ is
\begin{equation}
I(\mathcal{U};\mathcal{V})
=
\sum_{i=1}^{R}\sum_{j=1}^{C}
\frac{n_{ij}}{N}
\log\left(
\frac{n_{ij}/N}{(a_i/N)(b_j/N)}
\right),
\end{equation}
with entropies
\begin{equation}
H(\mathcal{U}) = -\sum_{i=1}^{R} \frac{a_i}{N}\log\frac{a_i}{N},
\qquad
H(\mathcal{V}) = -\sum_{j=1}^{C} \frac{b_j}{N}\log\frac{b_j}{N}.
\end{equation}
We use the arithmetic–mean normalized mutual information
(as in \texttt{sklearn}):
\begin{equation}
\mathrm{NMI}(\mathcal{U},\mathcal{V})
=
\frac{2 \, I(\mathcal{U};\mathcal{V})}{H(\mathcal{U}) + H(\mathcal{V})}.
\end{equation}
$\mathrm{NMI}$ ranges in $[0,1]$, where $1$ indicates that the two
partitions carry identical label information.

\subsection*{Homogeneity and Completeness}

Homogeneity measures whether each estimated cluster contains only members
of a single ground–truth class.  It is defined via the conditional entropy
of $\mathcal{U}$ given $\mathcal{V}$:
\begin{equation}
H(\mathcal{U}\mid\mathcal{V})
=
- \sum_{j=1}^{C}\sum_{i=1}^{R}
\frac{n_{ij}}{N}
\log
\frac{n_{ij}}{b_j},
\end{equation}
and
\begin{equation}
\mathrm{homogeneity}
=
1 - \frac{H(\mathcal{U}\mid\mathcal{V})}{H(\mathcal{U})}.
\end{equation}
Completeness measures whether all members of a given class are assigned
to the same cluster.  Using the conditional entropy of
$\mathcal{V}$ given $\mathcal{U}$,
\begin{equation}
H(\mathcal{V}\mid\mathcal{U})
=
- \sum_{i=1}^{R}\sum_{j=1}^{C}
\frac{n_{ij}}{N}
\log
\frac{n_{ij}}{a_i},
\end{equation}
we define
\begin{equation}
\mathrm{completeness}
=
1 - \frac{H(\mathcal{V}\mid\mathcal{U})}{H(\mathcal{V})}.
\end{equation}
Both scores lie in $[0,1]$; higher values indicate purer and more
coherent clusters, respectively.

\subsection*{V-measure}

The V-measure is the harmonic mean of homogeneity $h$ and completeness
$c$:
\begin{equation}
\mathrm{V\mbox{-}measure}
=
\frac{2 h c}{h + c},
\end{equation}
with $\mathrm{V\mbox{-}measure}=1$ if and only if both $h=1$ and $c=1$.

\subsection*{Silhouette Coefficient}

Let $d(\mathbf{x}_p,\mathbf{x}_q)$ be a distance between embedded points
(e.g.\ Euclidean distance).  For a point $i$ assigned to the cluster
$C(i)$, define
\begin{align}
a(i) &= \frac{1}{|C(i)|-1}
\sum_{\substack{j \in C(i)\\ j \neq i}}
d(\mathbf{x}_i,\mathbf{x}_j),
\\
b(i) &= \min_{C' \neq C(i)}
\frac{1}{|C'|}
\sum_{j \in C'} d(\mathbf{x}_i,\mathbf{x}_j),
\end{align}
where $a(i)$ is the average distance to points in the same cluster and
$b(i)$ is the minimum average distance to points in any other cluster.
The silhouette of point $i$ is
\begin{equation}
s(i)
=
\frac{b(i) - a(i)}{\max\{a(i), b(i)\}},
\end{equation}
and the overall silhouette coefficient is the mean over all points:
\begin{equation}
\mathrm{Silhouette}
=
\frac{1}{N} \sum_{i=1}^{N} s(i).
\end{equation}
The silhouette lies in $[-1,1]$, with values close to $1$ indicating
well-separated, compact clusters.

\FloatBarrier

\begin{table*}[pb]
    \centering
    \caption{Clustering quality of embedding spaces learned by Graph2Image (CNN-based) and graph neural networks (GNNs) on five datasets. Higher is better for all metrics.}
    \label{supp_tab:emb_metrics}
    \begin{tabular}{llrrrrrr}
        \toprule
        Dataset & Model & ARI & NMI & Homogeneity & Completeness & V-measure & Silhouette \\
        \midrule
        \multirow{4}{*}{PP-Pathways} 
            & GCN          & 0.032 & 0.137 & 0.146 & 0.129 & 0.137 & 0.115 \\
            & GAT          & 0.020 & 0.104 & 0.111 & 0.097 & 0.104 & 0.094 \\
            & GIN          & 0.009 & 0.037 & 0.022 & 0.113 & 0.037 & \textbf{0.850} \\
            & Graph2Image  & \textbf{0.176} & \textbf{0.497} & \textbf{0.527} & \textbf{0.470} & \textbf{0.497} & 0.054 \\
        \midrule
        \multirow{4}{*}{HuRI} 
            & GCN          & 0.092 & 0.184 & 0.176 & 0.193 & 0.184 & 0.145 \\
            & GAT          & 0.016 & 0.035 & 0.035 & 0.035 & 0.035 & 0.156 \\
            & GIN          & 0.035 & 0.018 & 0.015 & 0.022 & 0.018 & \textbf{0.523} \\
            & Graph2Image  & \textbf{0.281} & \textbf{0.475} & \textbf{0.480} & \textbf{0.469} & \textbf{0.475} & 0.140 \\
        \midrule
        \multirow{4}{*}{Pan} 
            & GCN          & 0.642 & 0.805 & 0.810 & 0.800 & 0.805 & 0.617 \\
            & GAT          & 0.626 & 0.768 & 0.776 & 0.760 & 0.768 & 0.425 \\
            & GIN          & 0.394 & 0.684 & 0.655 & 0.717 & 0.684 & 0.586 \\
            & Graph2Image  & \textbf{0.867} & \textbf{0.926} & \textbf{0.935} & \textbf{0.917} & \textbf{0.926} & 0.504 \\
        \midrule
        \multirow{4}{*}{TM} 
            & GCN          & \textbf{0.635} & 0.775 & 0.811 & 0.741 & 0.775 & 0.364 \\
            & GAT          & \textbf{0.634} & 0.786 & 0.812 & 0.761 & 0.786 & 0.320 \\
            & GIN          & 0.455 & 0.613 & 0.547 & 0.698 & 0.613 & 0.435 \\
            & Graph2Image  & 0.519 & \textbf{0.828} & \textbf{0.911} & \textbf{0.752} & \textbf{0.824} & 0.270 \\
        \midrule
        \multirow{4}{*}{Prostate Cancer} 
            & GCN          & 0.057 & 0.075 & 0.044 & 0.251 & 0.075 & 0.733 \\
            & GAT          & -0.008 & 0.000 & 0.000 & 0.000 & 0.000 & 0.483 \\
            & GIN          & 0.051 & 0.050 & 0.053 & 0.047 & 0.050 & 0.614 \\
            & Graph2Image  & \textbf{0.669} & \textbf{0.606} & \textbf{0.561} & \textbf{0.655} & \textbf{0.604} & \textbf{0.926} \\
        \bottomrule
    \end{tabular}
\end{table*}

\clearpage

\begin{figure}[pt]
    \centering
    \includegraphics[width=0.75\linewidth, page=21]{figures/Supplementary_Document_v2.pdf}
    \caption{
    t-SNE visualisation of embedding spaces learned by Graph2Image and graph neural network (GNN) baselines on the PP-Pathways interactome.
    Two-dimensional t-SNE projections of (a) Graph2Image (CNN-based) embedding, (b) GAT, (c) GCN and (d) GIN, coloured by GTEx tissue label. Graph2Image yields a markedly more structured and compact embedding space with discernible grouping of related tissues, whereas GNN baselines produce diffuse or overlapping manifolds with weaker separation. These differences indicate that Graph2Image captures tissue-specific expression patterns more coherently in the PP-Pathway protein–protein interaction network. The legend is provided in Figure~\ref{supp_figure:ppathway_embeddings_legend}.
    }
    \label{supp_figure:ppathway_embeddings}
\end{figure}

\begin{figure}[pt]
    \centering
    \includegraphics[width=0.8\linewidth, page=22]{figures/Supplementary_Document_v2.pdf}
    \caption{
    Legend for t-SNE visualisation of embedding spaces learned by Graph2Image and graph neural network for the PP-Pathways dataset.
    }
    \label{supp_figure:ppathway_embeddings_legend}
\end{figure}

\begin{figure}[pt]
    \centering
    \includegraphics[width=0.8\linewidth, page=23]{figures/Supplementary_Document_v2.pdf}
    \caption{
    t-SNE visualisation of embedding spaces learned by Graph2Image and graph neural network (GNN) baselines on the HuRI tissue dataset.
    Two-dimensional t-SNE projections of (a) Graph2Image (CNN-based) embedding, (b) GAT, (c) GCN and (d) GIN, coloured by GTEx tissue label. Graph2Image produces a substantially more organised and tissue-coherent embedding space, with smoother manifolds and clearer separation between major GTEx tissue groups. In contrast, the GNN baselines generate diffuse, intermingled, or fragmented structures, suggesting weaker preservation of tissue-specific transcriptomic signatures within the HuRI protein–protein network. The legend is provided in Figure~\ref{supp_figure:huri_embeddings}.
    }
    \label{supp_figure:huri_embeddings}
\end{figure}

\begin{figure}[pt]
    \centering
    \includegraphics[width=0.8\linewidth, page=24]{figures/Supplementary_Document_v2.pdf}
    \caption{
    Legend for t-SNE visualisation of embedding spaces learned by Graph2Image and graph neural network for the HuRI dataset.
    }
    \label{supp_figure:huri_embeddings_legend}
\end{figure}

\begin{figure}[pt]
    \centering
    \includegraphics[width=0.8\linewidth, page=25]{figures/Supplementary_Document_v2.pdf}
    \caption{
    t-SNE visualisation of embedding spaces learned by Graph2Image and graph neural network (GNN) baselines on the TM single-cell dataset. Two-dimensional t-SNE projections of (a) Graph2Image (CNN-based) embedding, (b) GAT, (c) GCN and (d) GIN, coloured by annotated cell type. Graph2Image produces compact, well-separated clusters that closely follow the biological annotations, whereas GNN embeddings often form elongated or partially overlapping manifolds, indicating a less label-consistent feature space. The legend is in Figure~\ref{supp_figure:tm_embeddings_legend}
    }
    \label{supp_figure:tm_embeddings}
\end{figure}

\begin{figure}[pt]
    \centering
    \includegraphics[width=0.8\linewidth, page=26]{figures/Supplementary_Document_v2.pdf}
    \caption{
    Legend for t-SNE visualisation of embedding spaces learned by Graph2Image and graph neural network for the TM dataset.
    }
    \label{supp_figure:tm_embeddings_legend}
\end{figure}

\begin{figure}[pt]
    \centering
    \includegraphics[width=0.8\linewidth, page=27]{figures/Supplementary_Document_v2.pdf}
    \caption{
    t-SNE visualisation of embedding spaces learned by Graph2Image and graph neural network (GNN) baselines on the Pan-cancer (Pan) cohort. Two-dimensional t-SNE projections of (a) Graph2Image (CNN-based) embedding, (b) GAT, (c) GCN and (d) GIN, coloured by tumour type. Graph2Image yields discrete, well-separated clusters for individual cancer types, while GNN embeddings exhibit stretched or interwoven manifolds with substantial overlap between tumours, consistent with reduced clustering purity. The legend is in Figure~\ref{supp_figure:pan_embeddings_legend}
    }
    \label{supp_figure:pan__embeddings}
\end{figure}

\begin{figure}[pt]
    \centering
    \includegraphics[width=0.5\linewidth, page=28]{figures/Supplementary_Document_v2.pdf}
    \caption{
    Legend for t-SNE visualisation of embedding spaces learned by Graph2Image and graph neural network for the Pan Cancer dataset.
    }
    \label{supp_figure:pan_embeddings_legend}
\end{figure}

\begin{figure}[pt]
    \centering
    \includegraphics[width=0.8\linewidth, page=29]{figures/Supplementary_Document_v2.pdf}
    \caption{
    t-SNE visualisation of embedding spaces learned by Graph2Image and graph neural network (GNN) baselines on the Prostate Cancer primary--metastasis cohort. Two-dimensional t-SNE projections of (a) Graph2Image (CNN-based) embedding, (b) GAT, (c) GCN and (d) GIN, coloured by clinical label (Primary vs.\ Metastasis). Graph2Image clearly separates primary tumours and metastatic lesions into disjoint clusters, whereas GNN embeddings show substantial mixing of the two labels and fragmented manifolds, indicating weaker alignment between the learned feature space and clinical outcomes.
    }
    \label{supp_figure:pnet_embeddings}
\end{figure}
